# Supplementary material for: X-MIC: Cross-Modal Instance Conditioning for Egocentric Action Generalization
Source: arXiv:2403.19811 source file (2024-03-28)
Supplement: Supplementary file 2 [file N_frames_supmat.tex]

\begin{table}
\centering
\scalebox{1}{
\centering
\setlength{\tabcolsep}{1.4mm}{
\resizebox{0.99\columnwidth}{!}{
\begin{tabular}{c|ccc|ccc}
\hline
\multirow{2}{*}{\# frames} & \multicolumn{3}{c|}{Nouns} & \multicolumn{3}{c}{Verbs} \\
\cline{2-7}
 & E4D & EK & hm & E4D & EK & hm \\
\hline
32 & 33.02 & 14.77 & 20.41 & 28.56 & 25.34 & 26.85 \\
16 & 33.54 & 15.35 & \textbf{21.06} & 28.93 & 26.48 & \textbf{27.65} \\
8 & 32.06 & 14.82 & 20.27 & 27.30 & 26.90 & 27.10 \\
4 & 31.74 & 14.99 & 20.36 & 26.41 & 26.17 & 26.29 \\
2 & 29.95 & 12.77 & 17.91 & 23.85 & 25.73 & 24.75 \\
\hline
\end{tabular}
}}}
\caption{\textbf{Influence of number of frames}. Trained on Ego4D. }
\label{tab:num_frames_supmat}
\vspace{-3mm}
\end{table}
